# Supplementary material for: Gas Adsorption and Dynamics in Pillared Graphene Frameworks
Source: arXiv:1707.00571 ancillary file (2017-07-03)
Supplement: Supplementary file 1 [file Gas_adsorption_in_pillared_graphene_frameworks_Supplementary_Info.pdf]

# Supplementary Information to the paper Gas Adsorption and Dynamics in Pillared Graphene Frameworks

Andrea Pedrielli[a,b], Simone Taioli[b,c,*], Giovanni Garberoglio[b,**], Nicola Maria Pugno[a,d,e]

[a]*Laboratory of Bio-Inspired and Graphene Nanomechanics, Department of Civil, Environmental and Mechanical Engineering, University of Trento, Via Mesiano 77, 38123 Trento, Italy*
[b]*European Centre for Theoretical Studies in Nuclear Physics and Related Areas (ECT*-FBK) and Trento Institute for Fundamental Physics and Applications (TIFPA-INFN), 38123 Trento, Italy*
[c]*Faculty of Mathematics and Physics, Charles University, 180 00 Prague 8, Czech Republic*
[d]*School of Engineering and Materials Science, Queen Mary University of London, Mile End Road, London E1 4NS, United Kingdom*
[e]*Ket Lab, Edoardo Amaldi Foudation, Italian Space Agency, Via del Politecnico snc, 00133 Rome, Italy*

*Second corresponding author
**First corresponding author
*Email addresses:* taioli@ectstar.eu (Simone Taioli), garberoglio@ectstar.eu (Giovanni Garberoglio)

*June 27, 2017*

## 1. Adsorption isotherms (DREIDING)

### *1.1. Pillar type 1*

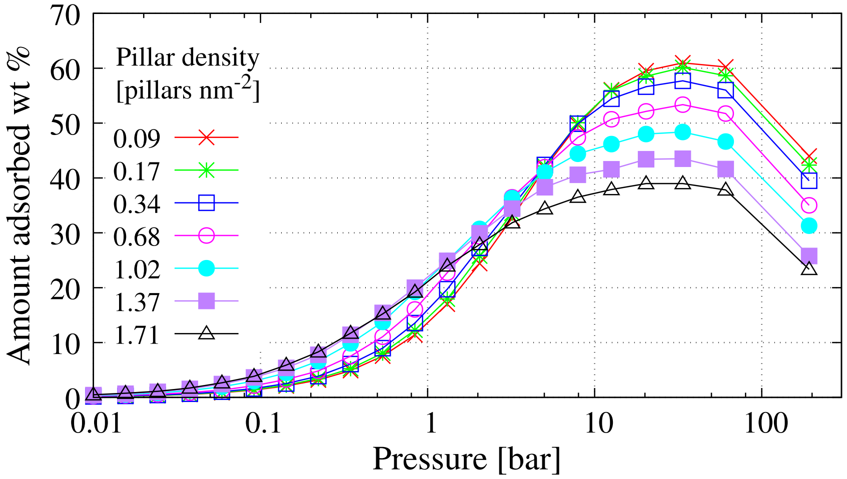


Figure 1: Gravimetric adsorption isotherms of $CO_2$ at T= 298 K for pillar type 1.

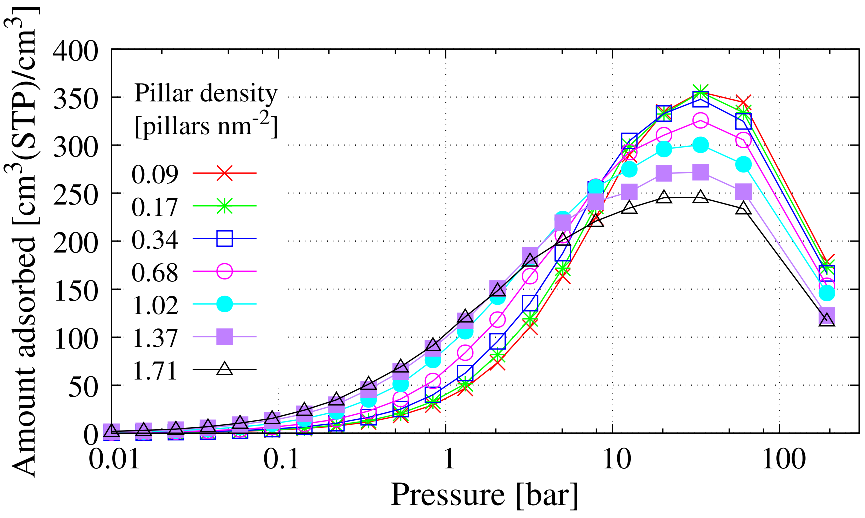


Figure 2: Volumetric adsorption isotherms of $CO_2$ at T= 298 K for pillar type 1.

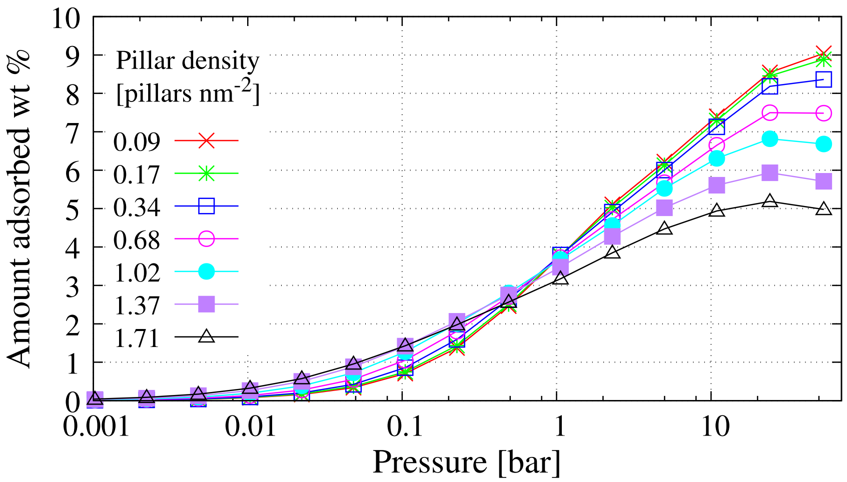


Figure 3: Gravimetric adsorption isotherms of $H_2$ at T= 77 K for pillar type 1.

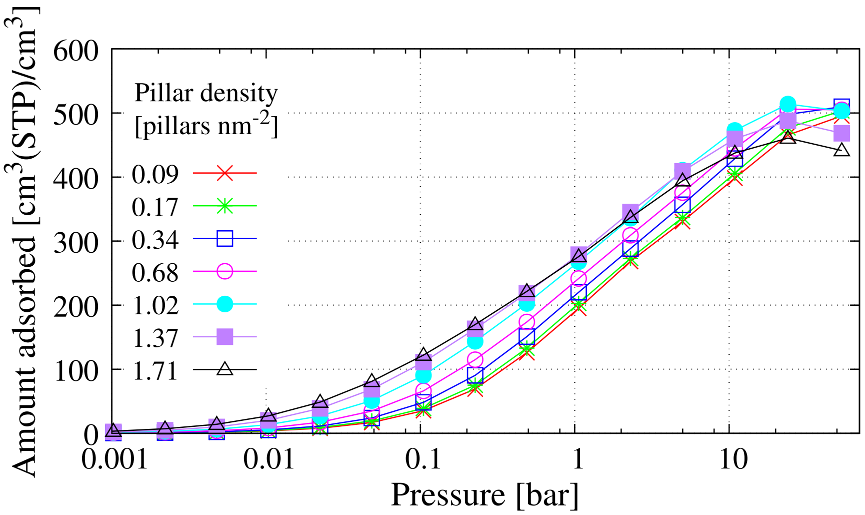


Figure 4: Volumetric adsorption isotherms of $H_2$ at T= 77 K for pillar type 1.

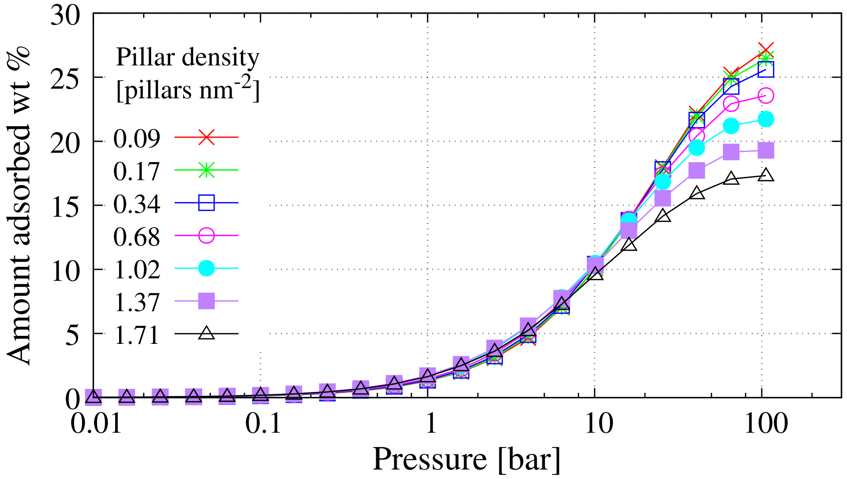


Figure 5: Gravimetric adsorption isotherms of $N_2$ at T= 298 K for pillar type 1.

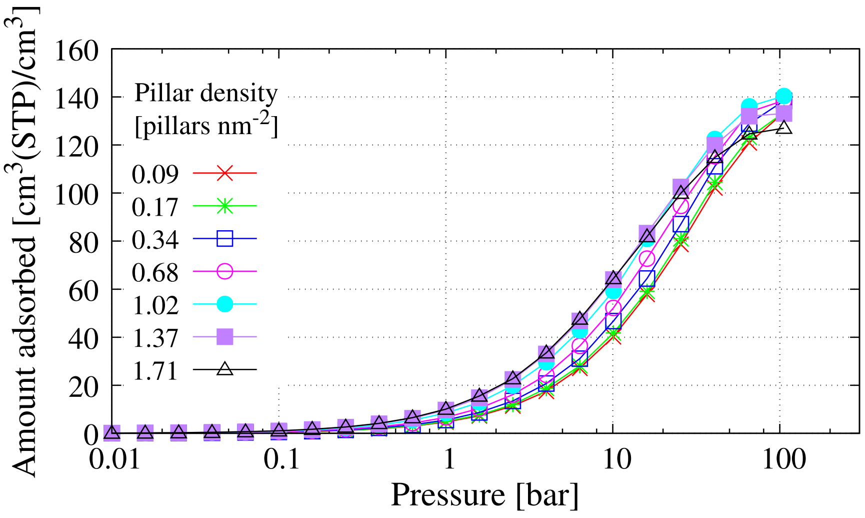


Figure 6: Volumetric adsorption isotherms of $N_2$ at T= 298 K for pillar type 1.

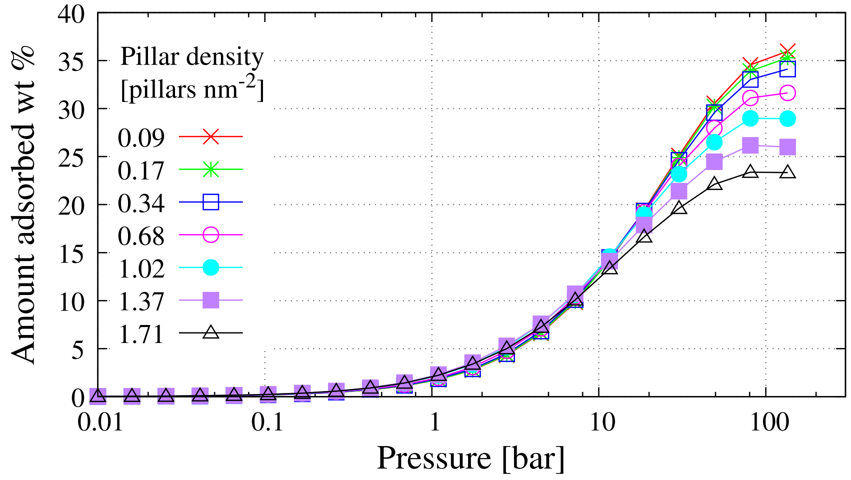


Figure 7: Gravimetric adsorption isotherms of $O_2$ at T= 298 K for pillar type 1.

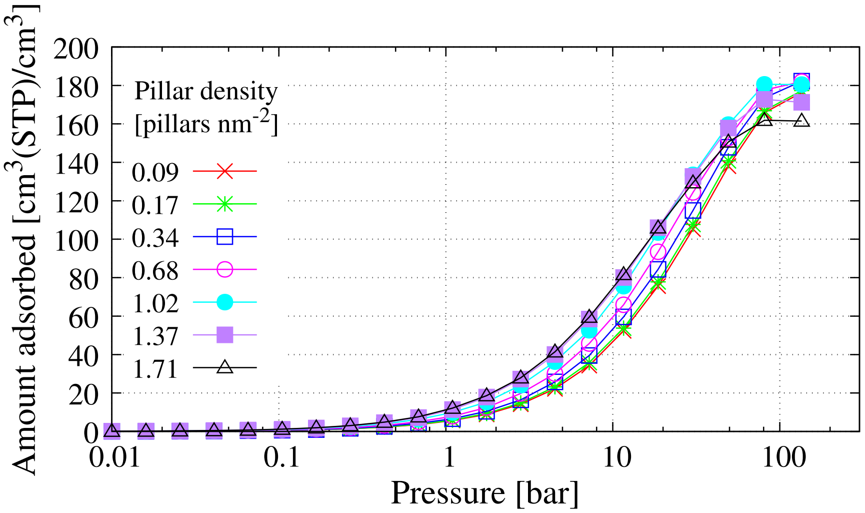


Figure 8: Volumetric adsorption isotherms of $O_2$ at T= 298 K for pillar type 1.

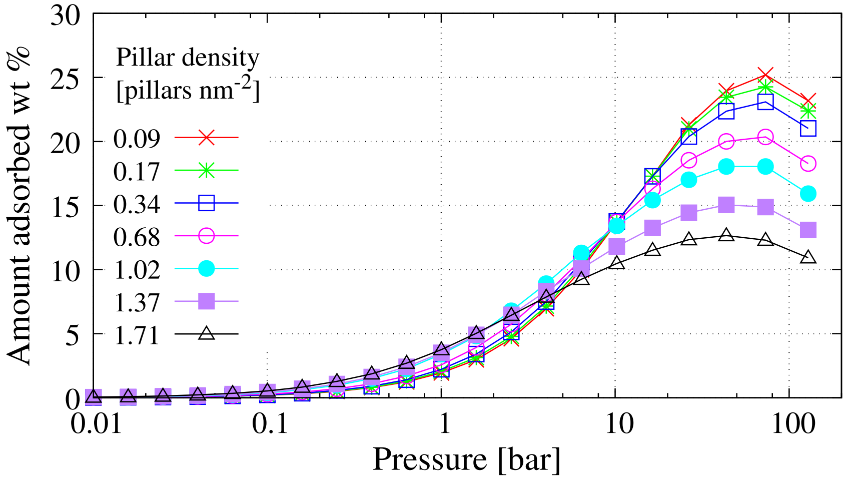


Figure 9: Gravimetric adsorption isotherms of $CH_4$ at T= 298 K for pillar type 2.

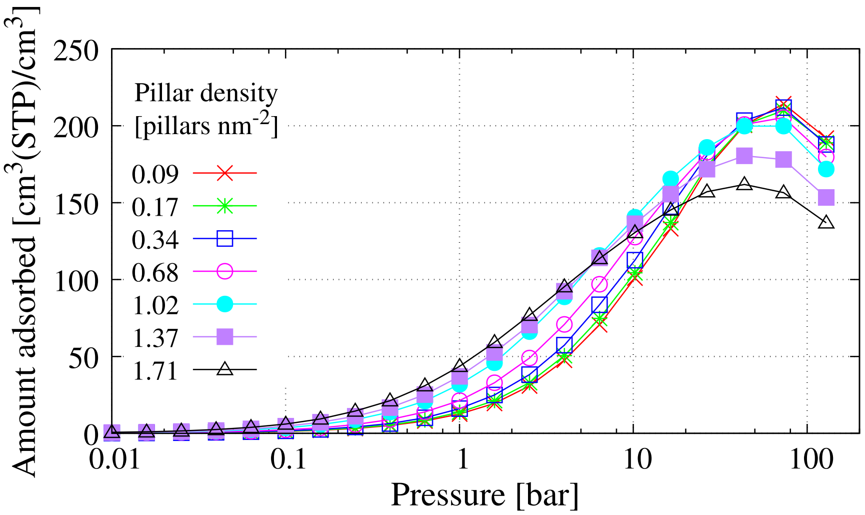


Figure 10: Volumetric adsorption isotherms of $CH_4$ at T= 298 K for pillar type 2.

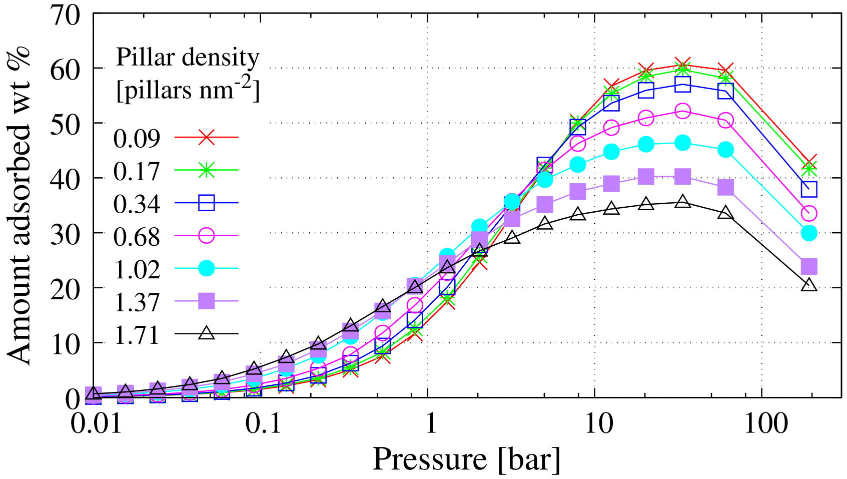


Figure 11: Gravimetric adsorption isotherms of $CO_2$ at T= 298 K for pillar type 2.

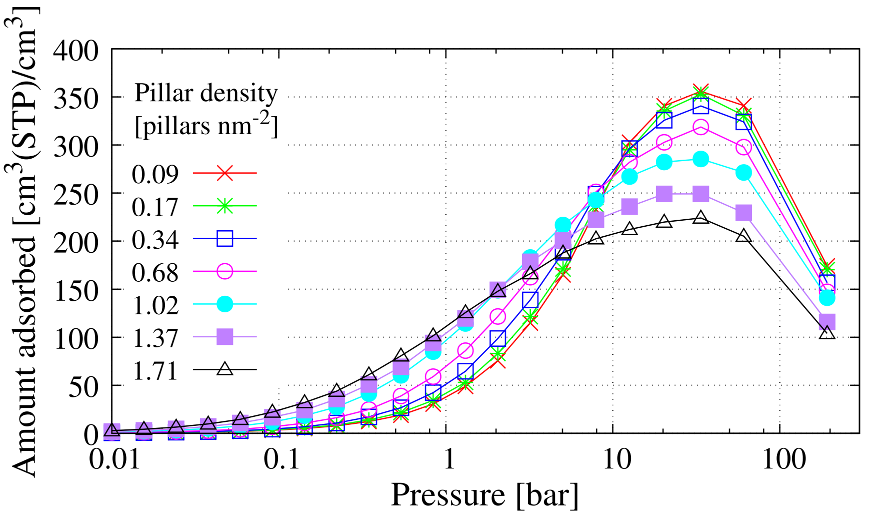


Figure 12: Volumetric adsorption isotherms of $CO_2$ at T= 298 K for pillar type 2.

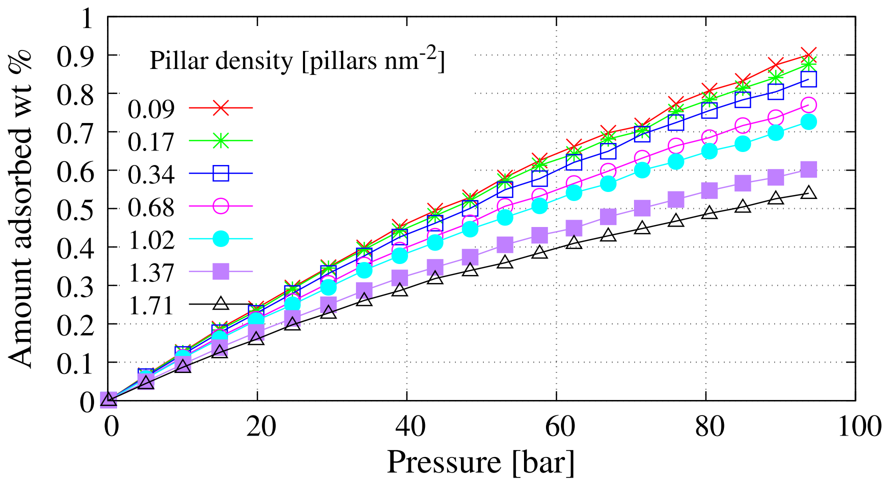


Figure 13: Gravimetric adsorption isotherms of $H_2$ at T= 298 K for pillar type 2.

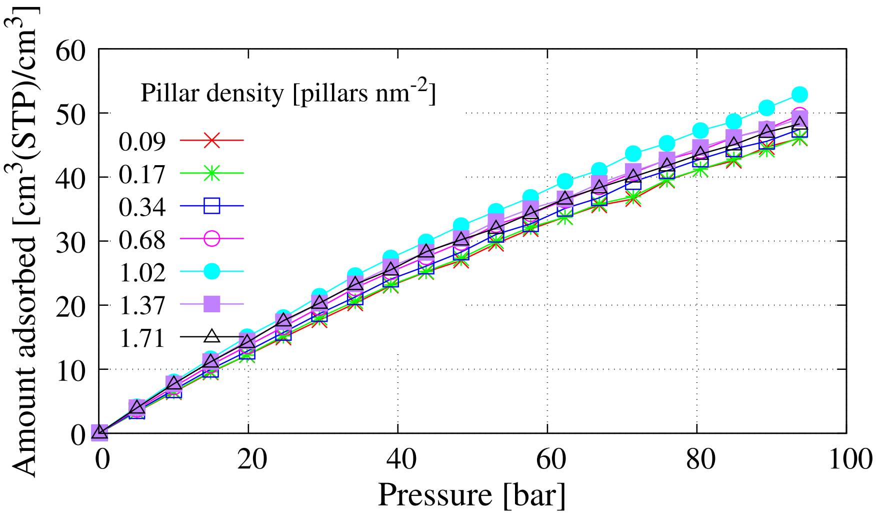


Figure 14: Volumetric adsorption isotherms of $H_2$ at T= 298 K for pillar type 2.

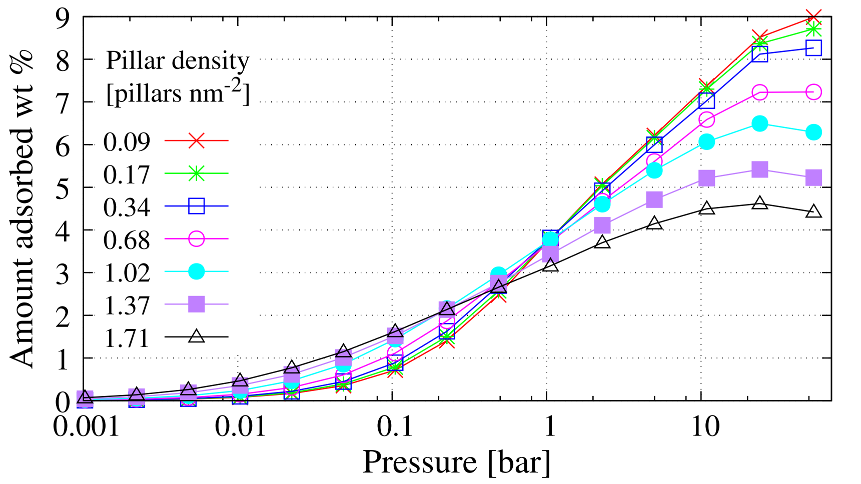


Figure 15: Gravimetric adsorption isotherms of $H_2$ at T= 77 K for pillar type 2.

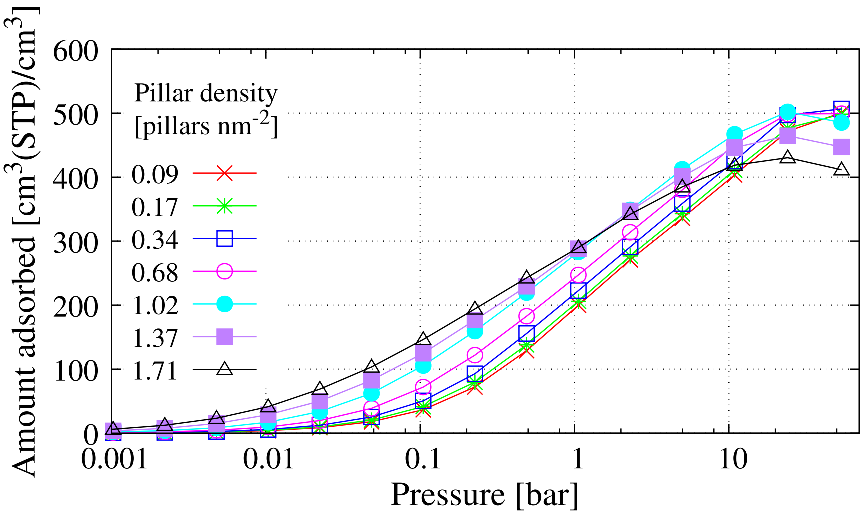


Figure 16: Volumetric adsorption isotherms of $H_2$ at T= 77 K for pillar type 2.

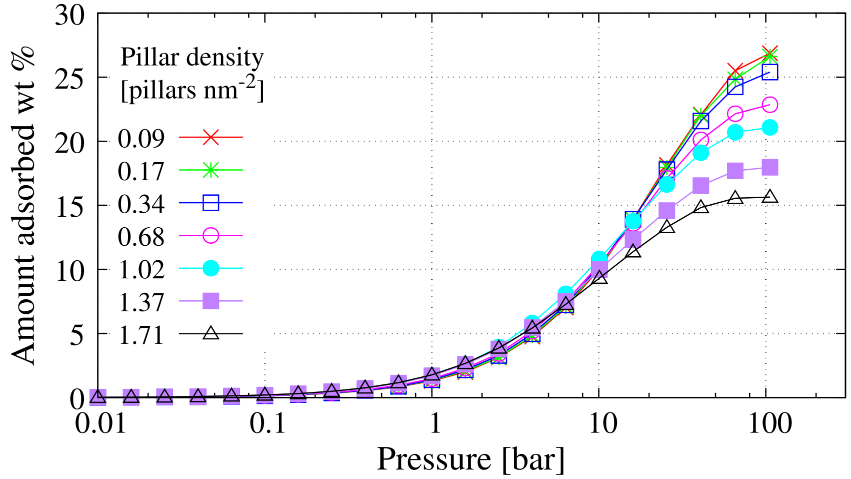


Figure 17: Gravimetric adsorption isotherms of $N_2$ at T= 298 K for pillar type 2.

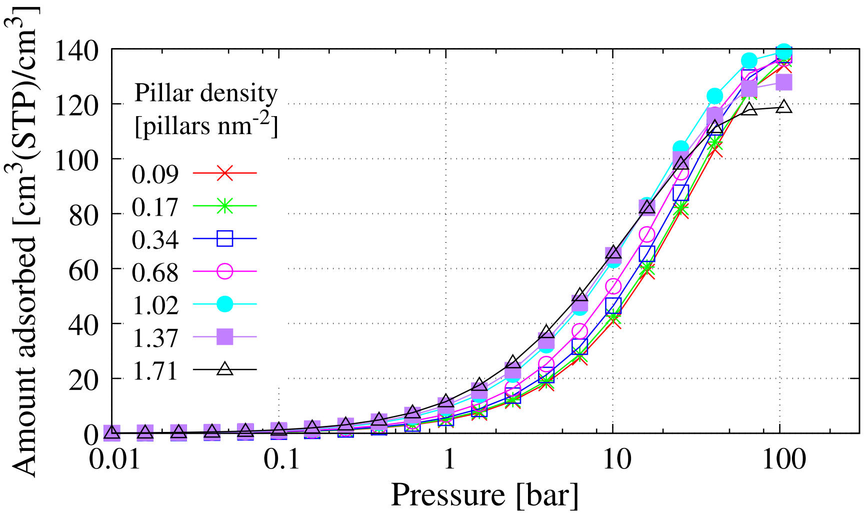


Figure 18: Volumetric adsorption isotherms of $N_2$ at T= 298 K for pillar type 2.

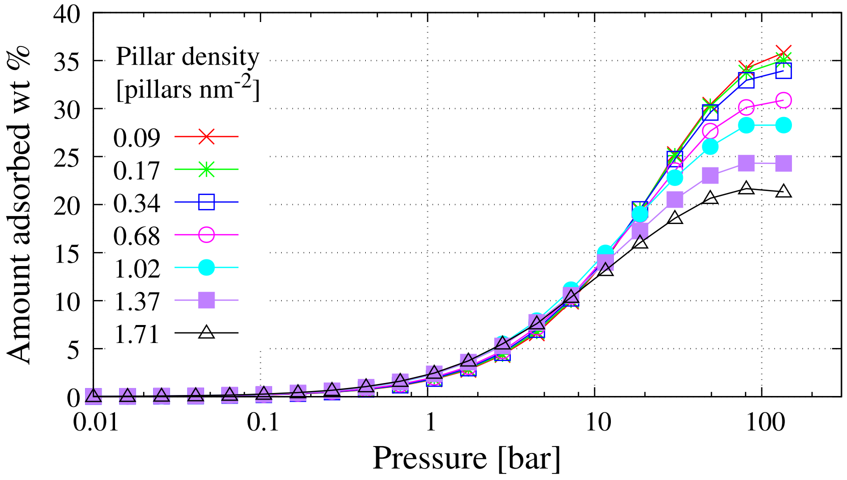


Figure 19: Gravimetric adsorption isotherms of $O_2$ at T= 298 K for pillar type 2.

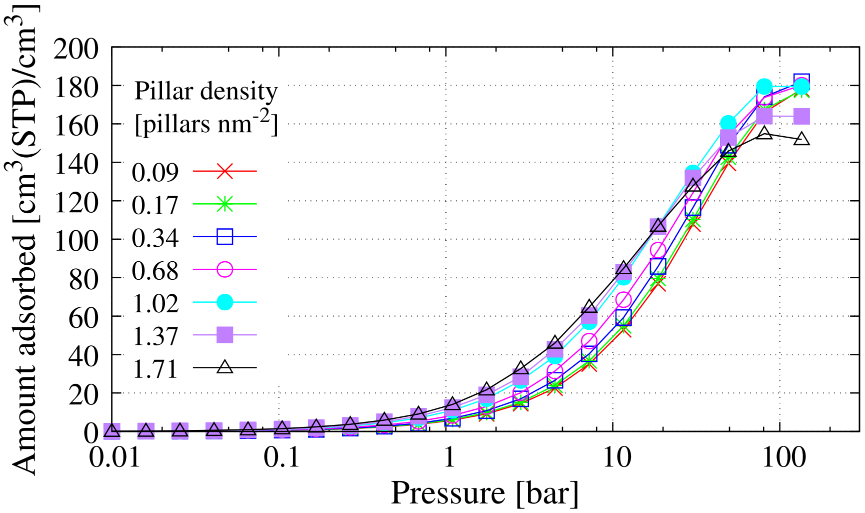


Figure 20: Volumetric adsorption isotherms of $O_2$ at T= 298 K for pillar type 2.

### 1.3. Pillar type 3

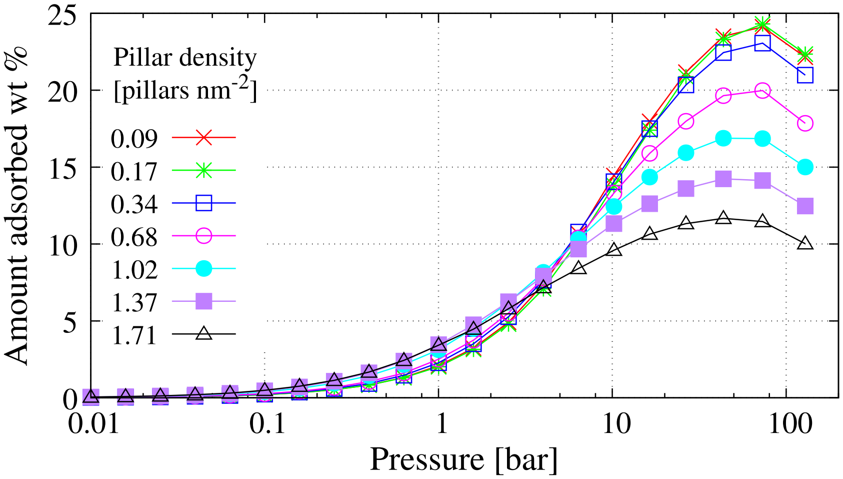


Figure 21: Gravimetric adsorption isotherms of $CH_4$ at T= 298 K for pillar type 3.

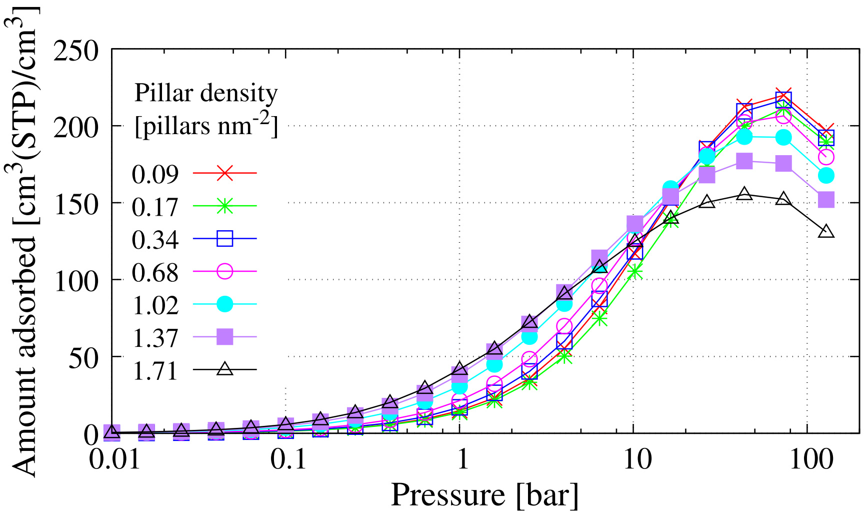


Figure 22: Volumetric adsorption isotherms of $CH_4$ at T= 298 K for pillar type 3.

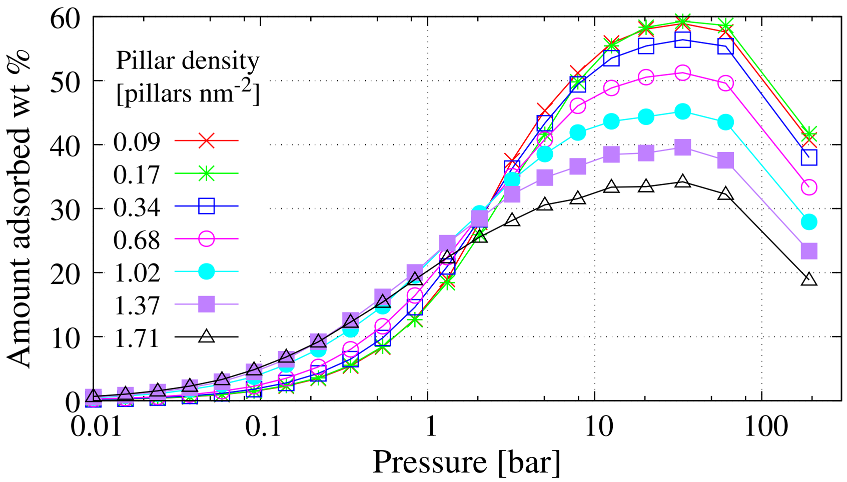


Figure 23: Gravimetric adsorption isotherms of $CO_2$ at T= 298 K for pillar type 3.

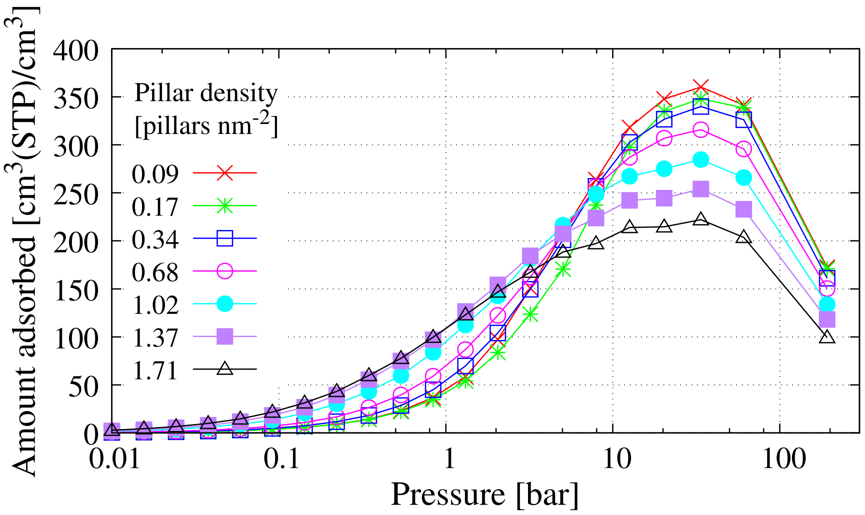


Figure 24: Volumetric adsorption isotherms of $CO_2$ at T= 298 K for pillar type 3.

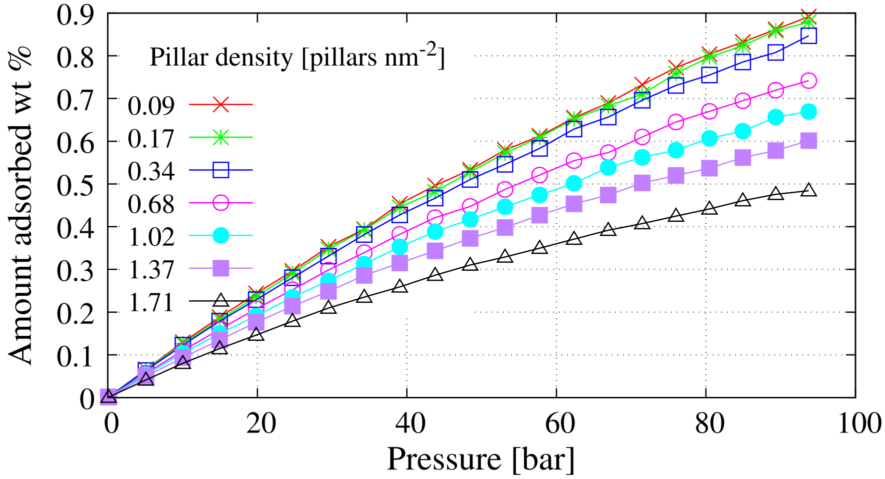


Figure 25: Gravimetric adsorption isotherms of $H_2$ at T= 298 K for pillar type 3.

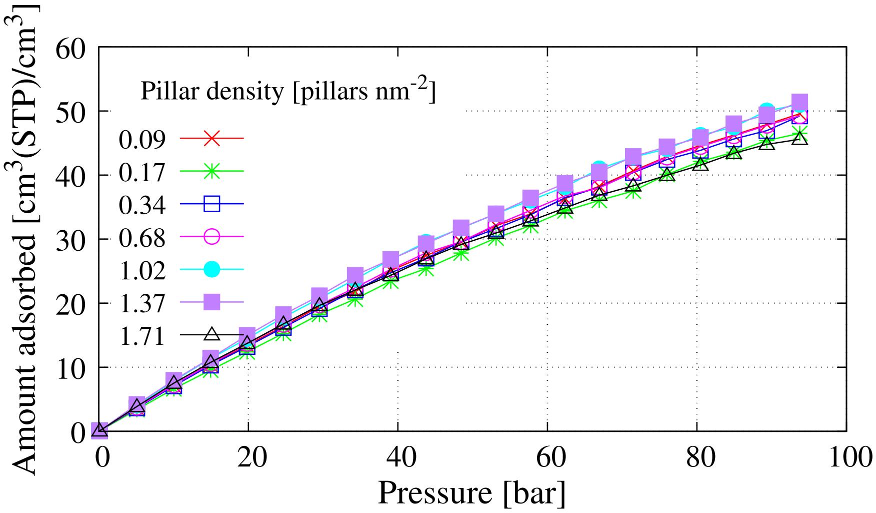


Figure 26: Volumetric adsorption isotherms of $H_2$ at T= 298 K for pillar type 3.

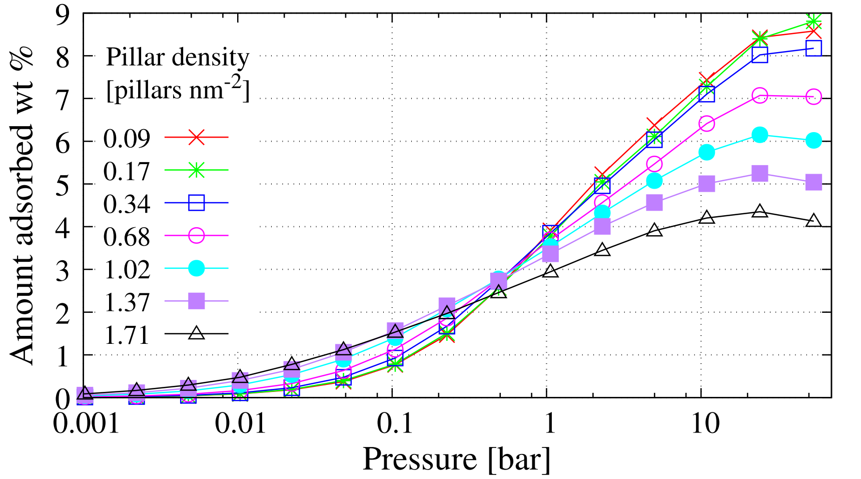


Figure 27: Gravimetric adsorption isotherms of $H_2$ at T= 77 K for pillar type 3.

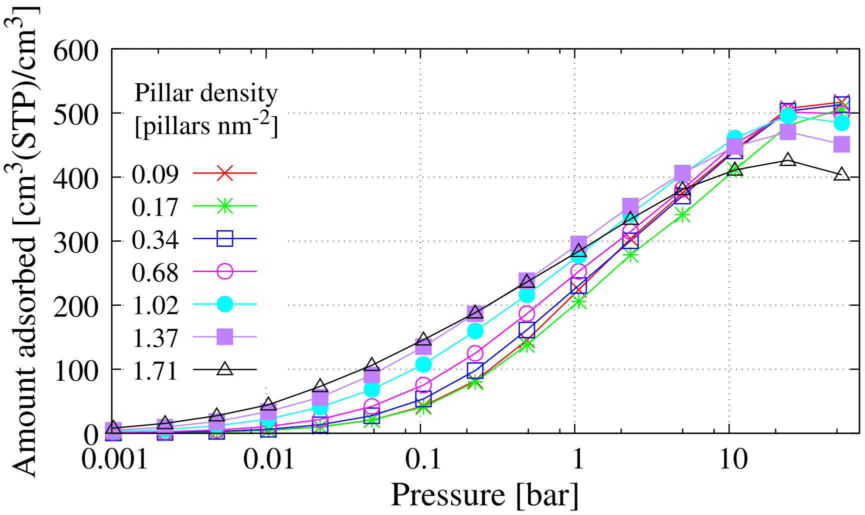


Figure 28: Volumetric adsorption isotherms of $H_2$ at T= 77 K for pillar type 3.

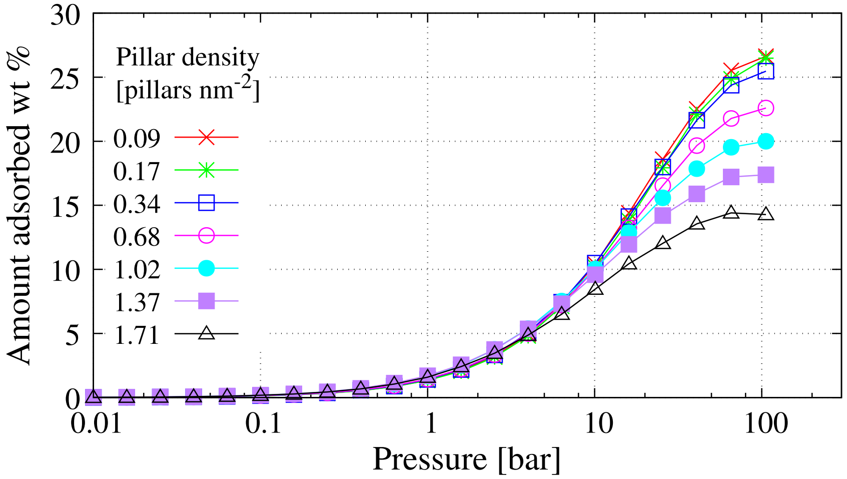


Figure 29: Gravimetric adsorption isotherms of $N_2$ at T= 298 K for pillar type 3.

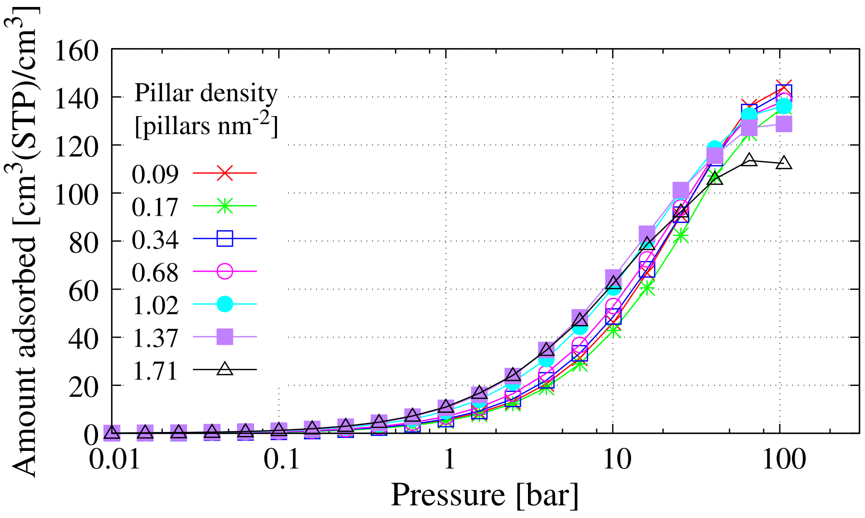


Figure 30: Volumetric adsorption isotherms of $N_2$ at T= 298 K for pillar type 3.

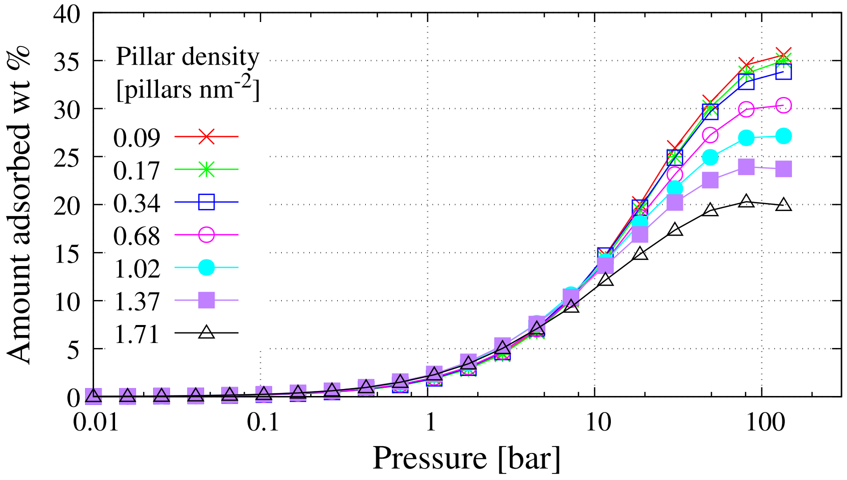


Figure 31: Gravimetric adsorption isotherms of $O_2$ at T= 298 K for pillar type 3.

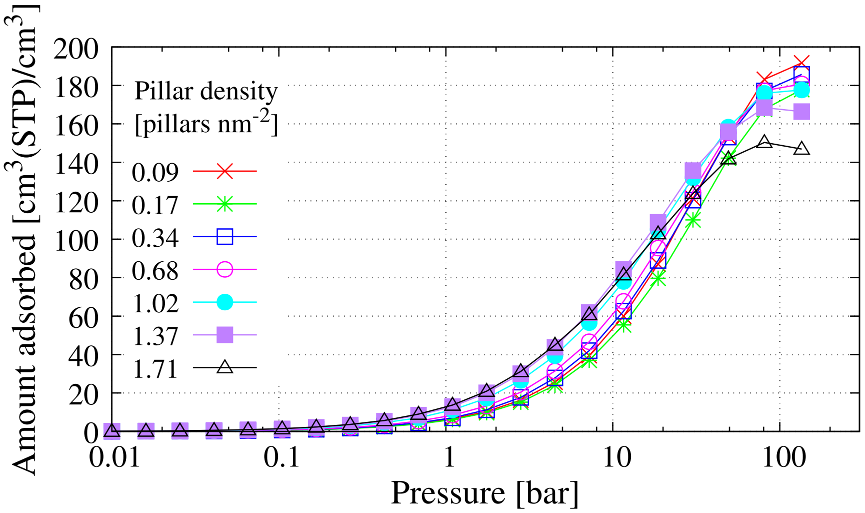


Figure 32: Volumetric adsorption isotherms of $O_2$ at T= 298 K for pillar type 3.

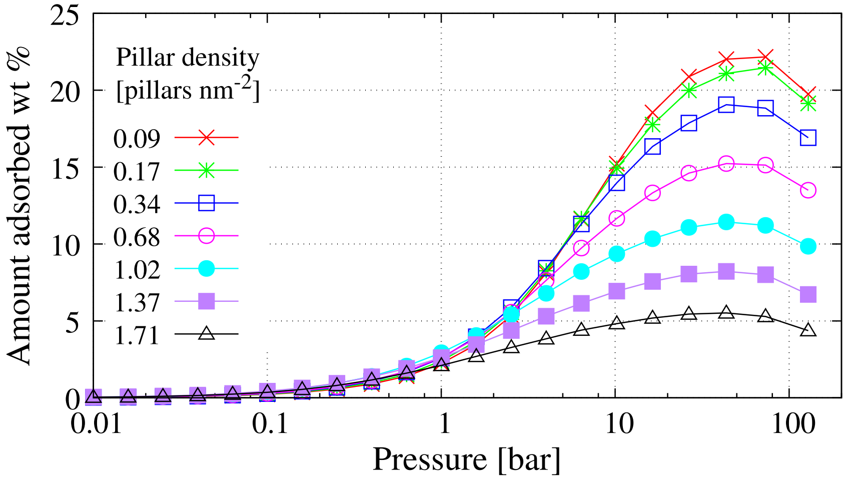


Figure 33: Gravimetric adsorption isotherms of $CH_4$ at T= 298 K for pillar type 4.

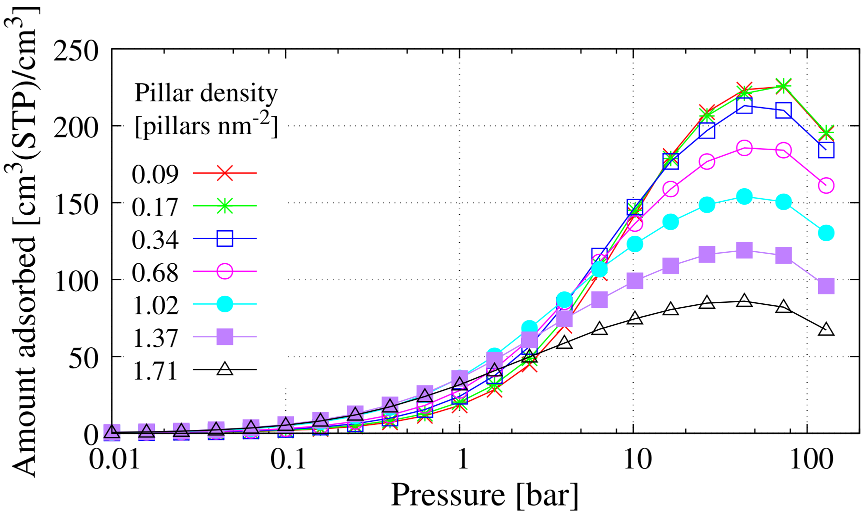


Figure 34: Volumetric adsorption isotherms of $CH_4$ at T= 298 K for pillar type 4.

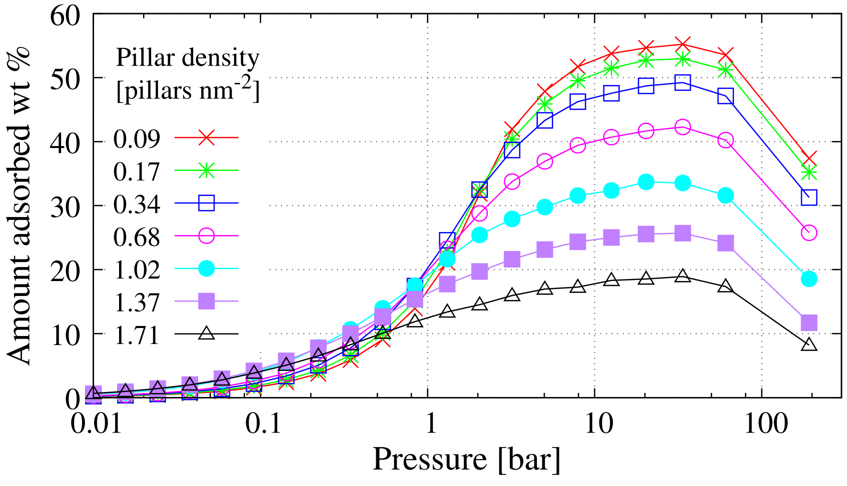


Figure 35: Gravimetric adsorption isotherms of $CO_2$ at T= 298 K for pillar type 4.

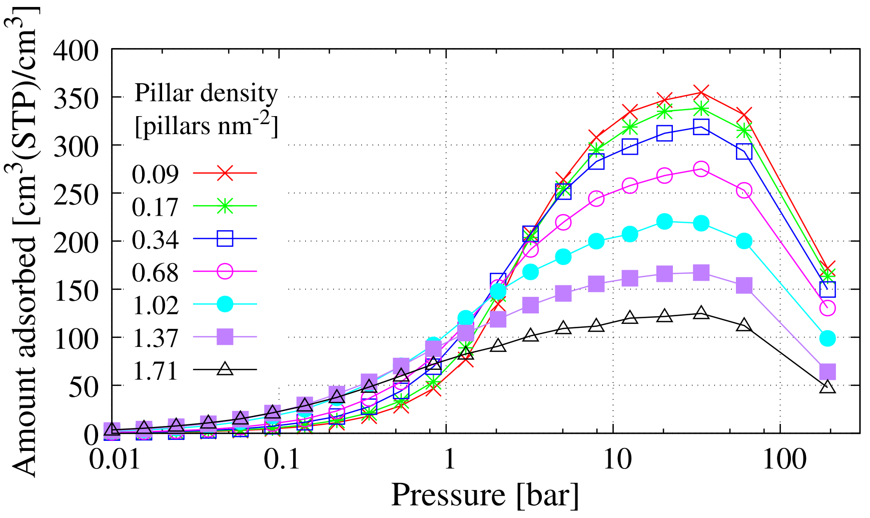


Figure 36: Volumetric adsorption isotherms of $CO_2$ at T= 298 K for pillar type 4.

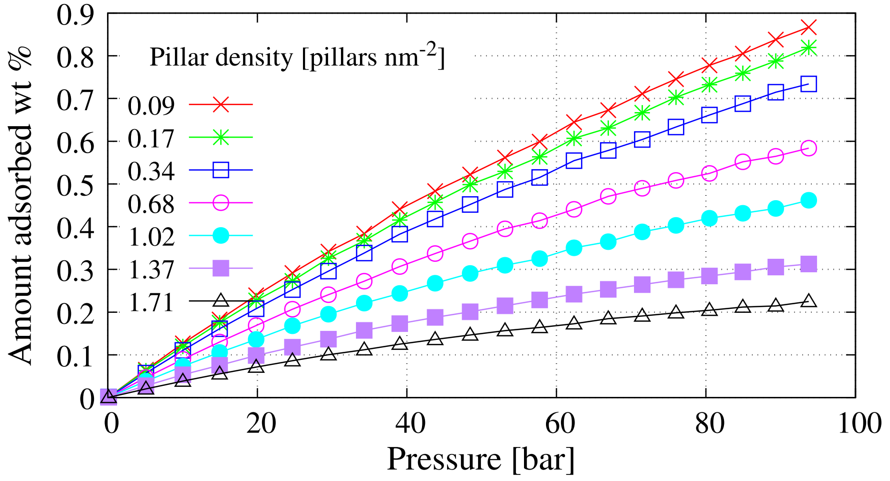


Figure 37: Gravimetric adsorption isotherms of $H_2$ at T= 298 K for pillar type 4.

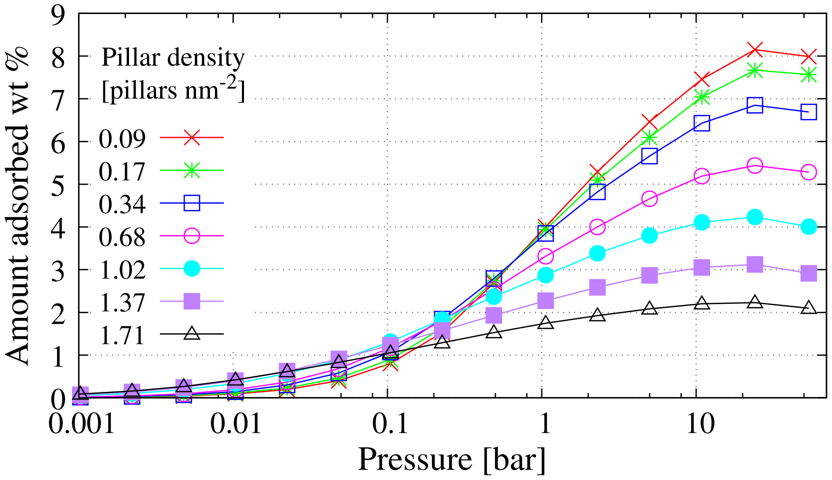


Figure 38: Gravimetric adsorption isotherms of $H_2$ at T= 77 K for pillar type 4.

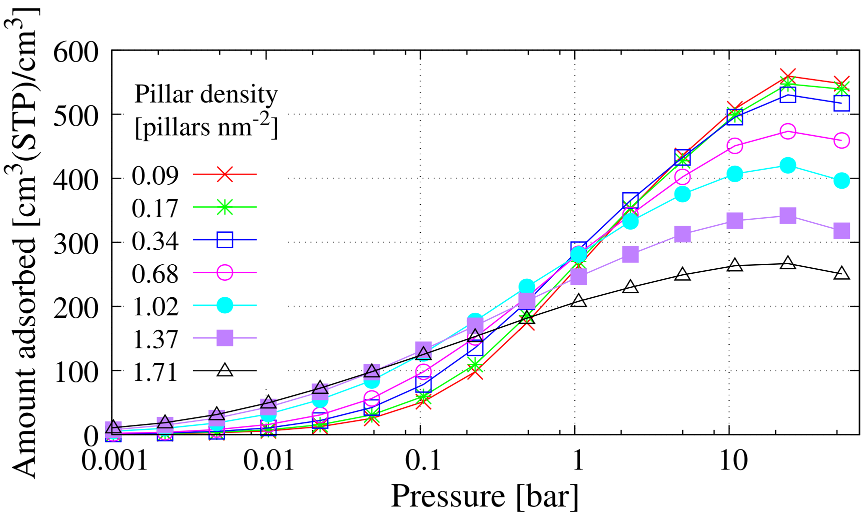


Figure 39: Volumetric adsorption isotherms of $H_2$ at T= 77 K for pillar type 4.

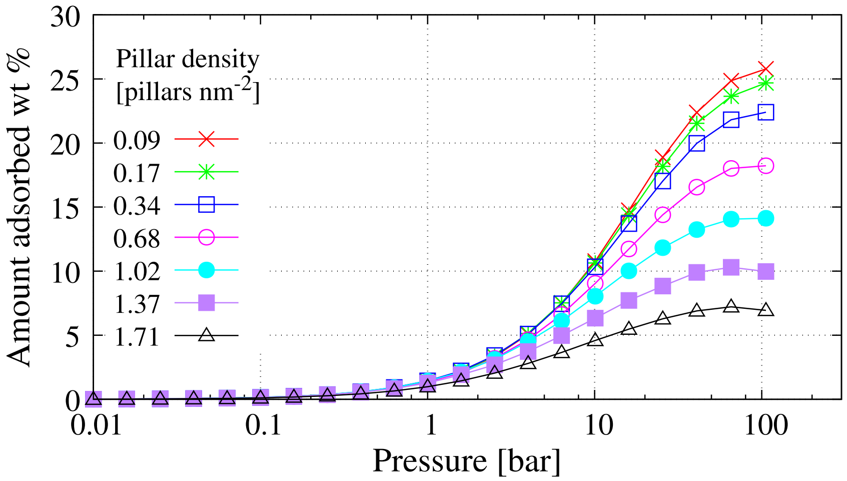


Figure 40: Gravimetric adsorption isotherms of $N_2$ at T= 298 K for pillar type 4.

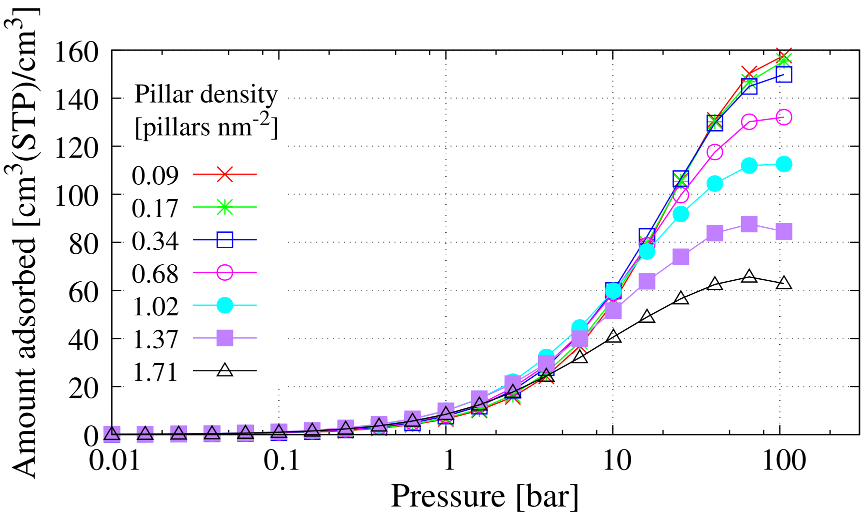


Figure 41: Volumetric adsorption isotherms of $N_2$ at T= 298 K for pillar type 4.

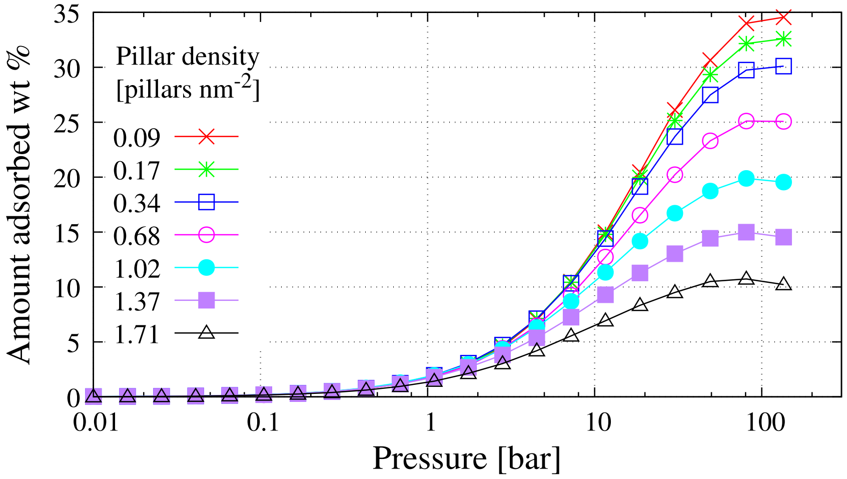


Figure 42: Gravimetric adsorption isotherms of $O_2$ at T= 298 K for pillar type 4.

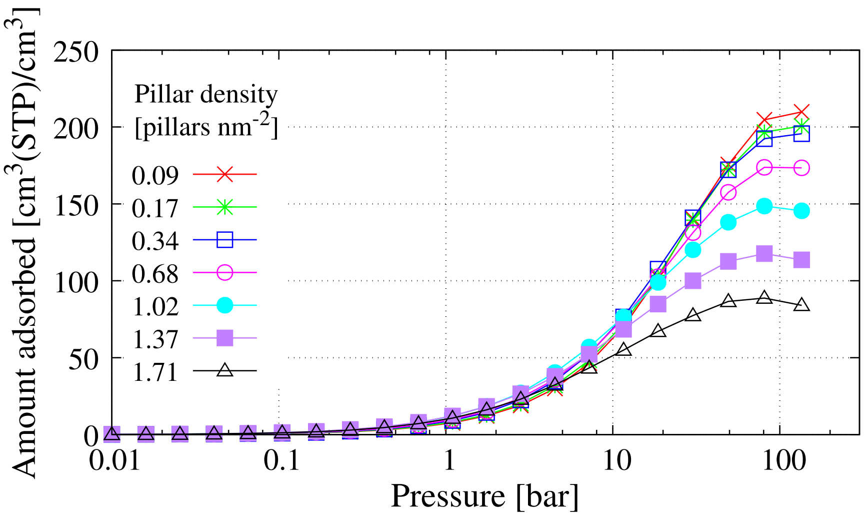


Figure 43: Volumetric adsorption isotherms of $O_2$ at T= 298 K for pillar type 4.

## 2. UFF vs DREIDING, Relative overestimation R

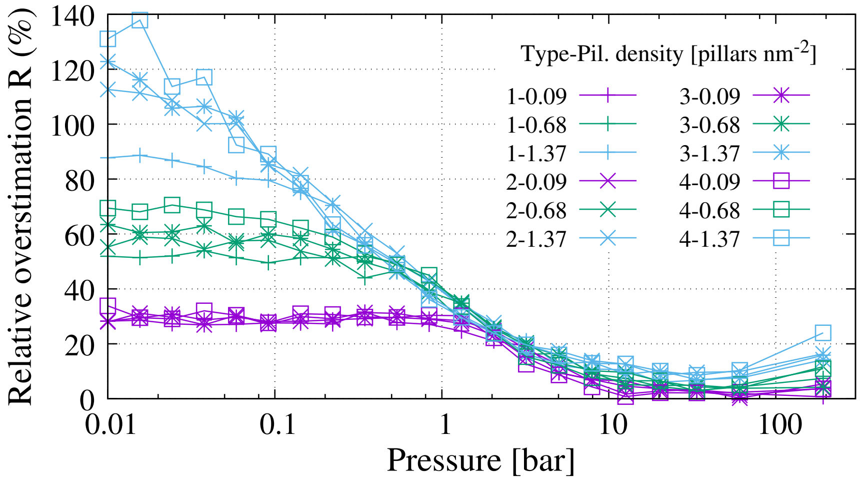


Figure 44: Relative overestimation $R$ of $CO_2$ adsorption at 298 K using UFF force field in place of DREIDING force field.

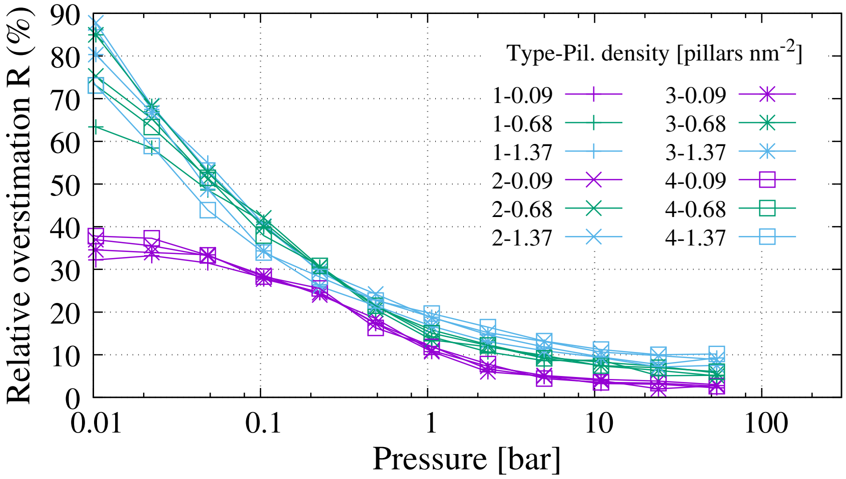


Figure 45: Relative overestimation $R$ of $H_2$ adsorption at 77 K using UFF force field in place of DREIDING force field.

## 3. Selectivity (DREIDING)

### *3.1. Pillar type 1*

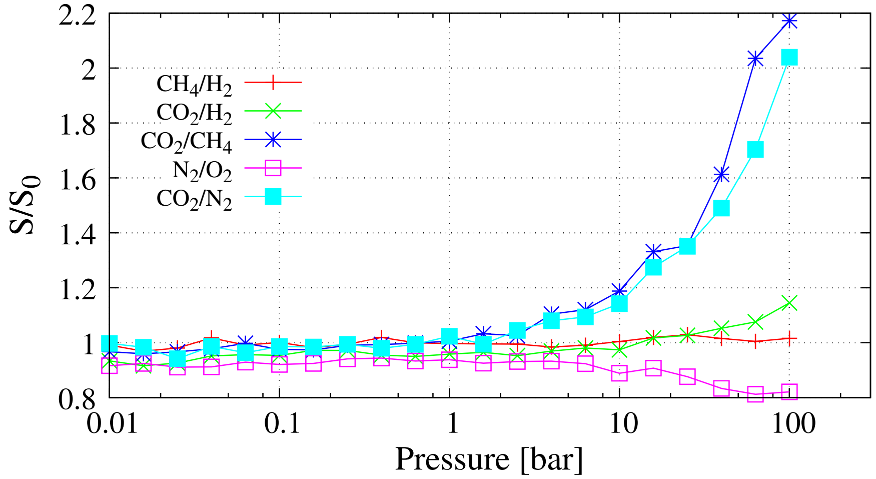


Figure 46: Selectivity for gas mixtures at T= 298 K, normalized with respect to the zero-pressure limit value of selectivity ($S_0$), for the sample with pillar type 1 and pillar density 0.09 pillars nm $^{-2}$.

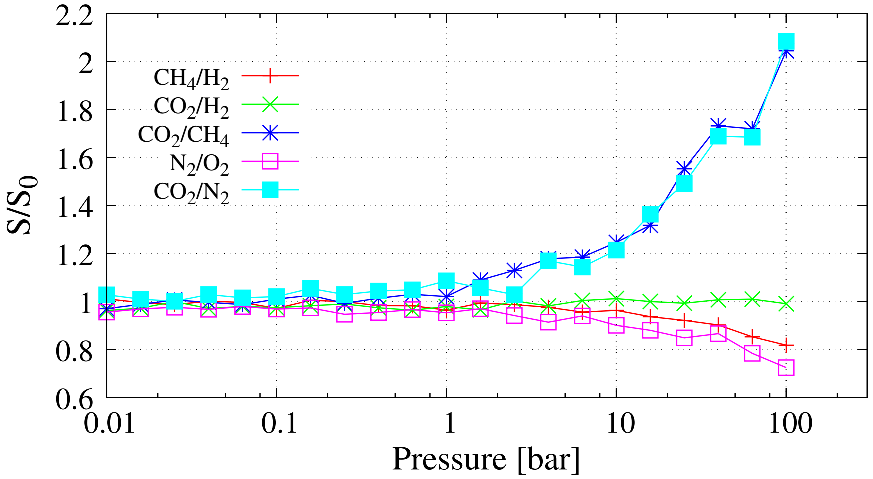


Figure 47: Selectivity for gas mixtures at T= 298 K, normalized with respect to the zero-pressure limit value of selectivity ($S_0$), for the sample with pillar type 1 and pillar density 1.37 pillars nm $^{-2}$.

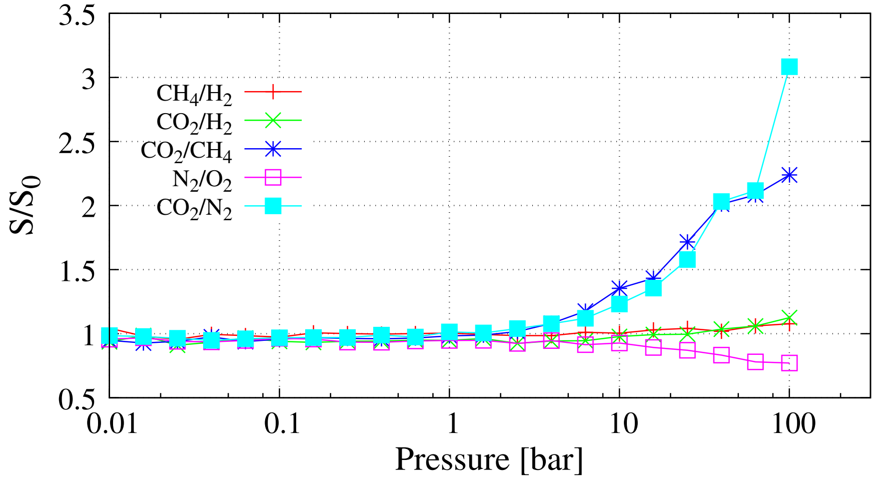


Figure 48: Selectivity for gas mixtures at T= 298 K, normalized with respect to the zero-pressure limit value of selectivity ($S_0$), for the sample with pillar type 4 and pillar density 0.09 pillars nm $^{-2}$.

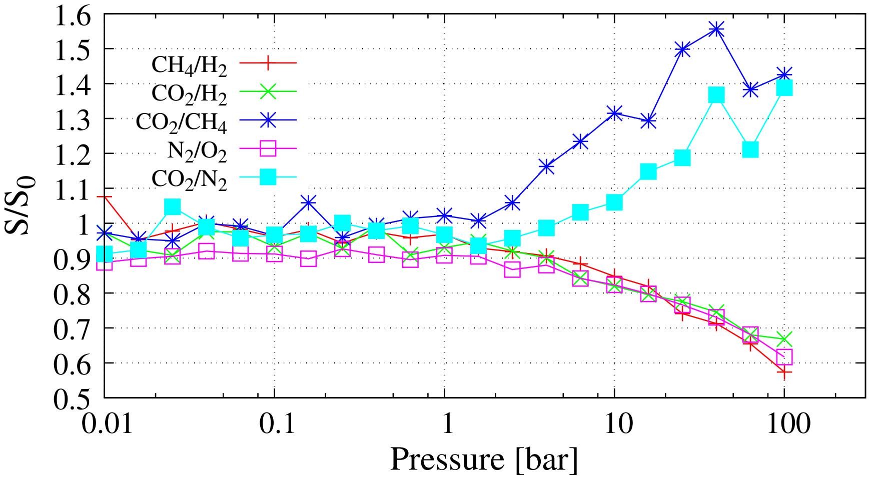


Figure 49: Selectivity for gas mixtures at T= 298 K, normalized with respect to the zero-pressure limit value of selectivity ($S_0$), for the sample with pillar type 4 and pillar density 1.37 pillars nm $^{-2}$.
